# Supplementary material for: The Erd\H{o}s-Straus conjecture New modular equations and checking up to $N=10^{17}$
Source: arXiv:1406.6307 ancillary file (2014-06-24)
Supplement: Supplementary file 1 [file erdos_straus_fr.pdf]

# Conjecture d'Erdős-Straus

## Nouvelles équations modulaires et vérification jusqu'à $N = 10^{17}$

Serge E. SALEZ

24 juin 2014

### Résumé

En 1999 Allan Swett [5] vérifia (en 150 heures) la conjecture d'Erdős-Straus jusqu'à  $N = 10^{14}$  à l'aide d'un crible construit sur une unique équation modulaire. Après avoir démontré l'existence d'un ensemble "complet" de sept équations modulaires (dont trois nouvelles), ce papier propose un crible optimisé construit sur ces équations. Un programme écrit en C++ (et donné par ailleurs) permet alors d'effectuer la vérification en des temps allant, sur un ordinateur basique<sup>1</sup>, de quelques minutes pour  $N = 10^{14}$  à environ 16 heures pour  $N = 10^{17}$ .

## 1 Formules de base

On dira qu'une fraction est  $k$ -égyptienne si elle est la somme d'au plus  $k$  fractions positives unitaires (c'est-à-dire de numérateur 1). La conjecture d'Erdős-Straus consiste à dire que la fraction  $4/n$  est 3-égyptienne pour tout  $n > 1$ .

### 1.1 Réduction

Grâce aux identités

$$\frac{1}{t} = \frac{1}{t+1} + \frac{1}{t(t+1)}$$

et

$$\frac{2}{2t-1} = \frac{1}{t} + \frac{1}{t(2t-1)}$$

il est équivalent (pour  $n > 2$ ) d'imposer une écriture avec *exactement* 3 fractions unitaires *distinctes*, ce que l'on fera par la suite.

D'autre part, les identités

$$\frac{4}{3t-1} = \frac{1}{t} + \frac{1}{3t-1} + \frac{1}{t(3t-1)}$$

$$\frac{4}{4t-1} = \frac{1}{t} + \frac{1}{t(4t-1)}$$

$$\frac{4}{8t-3} = \frac{1}{2t} + \frac{1}{t(8t-3)} + \frac{1}{2t(8t-3)}$$

montrent que la conjecture est vérifiée si  $n \equiv -1 \pmod{3}$  ou  $n \equiv -1 \pmod{4}$  ou  $n \equiv -3 \pmod{8}$ . De plus, si  $4/n$  est 3-égyptienne alors  $4/kn$  l'est aussi.

*Conclusion* : Il suffit de démontrer que  $4/p$  est 3-égyptienne, pour tout nombre premier  $p$  vérifiant  $p \equiv 1 \pmod{24}$ .

---

1. AMD TurionII Dual-Core Mobile M250 (64 bits, 16 100 MIPS).

## 1.2 Formules de Rosati

La proposition suivante est due (d'après Mordell<sup>2</sup>) à Rosati [3]. La démonstration est élémentaire et a été maintes fois reproduite. Celle ci-dessous est néanmoins originale et uniformise les notations.

On note  $\mathcal{A} = \mathbb{Z}$  et  $\mathcal{A}_+$  l'ensemble des éléments strictement positifs de  $\mathbb{Z}$ . Dans ce contexte, on appelle *élément premier* un nombre premier impair.

PROPOSITION 1 *Soit  $p$  un élément premier. La fraction  $4/p$  est 3-égyptienne si et seulement si il existe quatre éléments de  $\mathcal{A}_+$  notés  $A, B, C, D$  vérifiant*

$$4ABCD = A + B + pC \quad \text{et} \quad (ABD, p) = 1 \quad (1)$$

ou

$$4ABCD = p(A + B) + C \quad \text{et} \quad (ABCD, p) = 1 \quad (2)$$

DÉMONSTRATION Puisque  $4/p$  est 3-égyptienne, il existe 3 éléments de  $\mathcal{A}_+$  notés  $X_1, X_2, X_3$  tels que

$$\frac{4}{p} = \frac{1}{X_1} + \frac{1}{X_2} + \frac{1}{X_3} \quad (3)$$

Les  $X_i$  ne sont pas tous divisibles par  $p$  car sinon on aurait

$$4 = \frac{1}{X_1/p} + \frac{1}{X_2/p} + \frac{1}{X_3/p} \leq 3$$

De (3) on déduit

$$4X_1X_2X_3 = p(X_2X_3 + X_3X_1 + X_1X_2)$$

ce qui montre que  $p$  divise l'un au moins des  $X_i$ . On peut donc poser (éventuellement en renumérotant les  $X_i$ )  $x_i = X_i/p_i$  avec

$$p_1 = p_2 = 1, \quad p_3 = p \quad \text{et} \quad (x_1x_2, p) = 1$$

ou

$$p_1 = p_2 = p, \quad p_3 = 1 \quad \text{et} \quad (x_3, p) = 1$$

suivant que  $p$  divise exactement un ou deux  $X_i$ .

on obtient alors (puisque  $p_2p_3 = p$ )

$$4p_1p x_1x_2x_3 = p(p_2p_3x_2x_3 + p_3p_1x_3x_1 + p_1p_2x_1x_2)$$

D'où

$$4x_1x_2x_3 = p_3x_2x_3 + p_3x_3x_1 + p_2x_1x_2$$

En posant  $D = (x_1, x_2, x_3)$  et  $x'_i = x_i/D$  on obtient

$$4Dx'_1x'_2x'_3 = p_3x'_2x'_3 + p_3x'_3x'_1 + p_2x'_1x'_2$$

On pose enfin

$$A = (x'_2, x'_3), \quad B = (x'_3, x'_1), \quad C = (x'_1, x'_2)$$

Puisque  $(x'_1, x'_2, x'_3) = 1$  alors  $A, B, C$  sont deux à deux premiers entre eux. On en déduit qu'il existe des éléments  $t_i \in \mathcal{A}_+$  deux à deux premiers entre eux tels que

$$x'_1 = BCt_1, \quad x'_2 = CA t_2, \quad x'_3 = AB t_3$$

On remarque que

$$(t_1, A) = (t_2, B) = (t_3, C) = 1$$

Avec ces notations

$$4D BC CA AB t_1 t_2 t_3 = p_3 CA AB t_2 t_3 + p_3 AB BC t_3 t_1 + p_2 BC CA t_1 t_2$$

---

2. Ainsi, contrairement à la plupart des articles, nous n'attribuons pas à Mordell ce que Mordell lui même attribue à d'autres mathématiciens. Dans son livre [2], souvent cité, les quatre pages qu'il consacre à cette conjecture ne présentent pas une étude personnelle mais relatent succinctement quelques travaux dont les sources sont soigneusement indiquées : il est donc tout à fait erroné de parler de "théorème de Mordell" ou de "formules de Mordell". Toute proportion gardée, il ne faudrait pas reproduire ce qui s'est passé avec l'équation de Pell.

et donc

$$4ABCDt_1t_2t_3 = p_3At_2t_3 + p_3Bt_3t_1 + p_2Ct_1t_2$$

De  $t_1 \mid p_3At_2t_3$  on déduit  $t_1 \mid p_3$  et donc  $t_1 = 1$  puisque  $(x_1, p_3) = 1$ . De même  $t_2 = 1$  et  $t_3 = 1$ . D'où

$$4ABCD = p_3A + p_3B + p_2C \quad (4)$$

Réciproquement, si les nombres  $A, B, C, D$  vérifient la relation (4) alors en divisant par  $pABCD$  on obtient

$$\frac{4}{p} = \frac{1}{p_1BCD} + \frac{1}{p_2ACD} + \frac{1}{p_3ABD}$$

ce qui montre que  $4/p$  est 3-égyptienne<sup>3</sup>. ■

*Remarque :* Si  $p$  n'est pas premier, la relation (4) est encore *suffisante* mais elle n'est plus *nécessaire*.

### 1.3 Notations

Par la suite, nous utiliserons systématiquement les notations de la Proposition 1. On introduit de plus deux nouveaux éléments de  $\mathcal{A}_+$  notés  $E$  et  $F$ .

D'après (4) on a  $C \mid A + B$  puisque  $(C, p_3) = 1$ . Si on pose  $E = (A + B)/C$  alors  $E \in \mathcal{A}_+$  et (4) est équivalent à

$$\begin{cases} 4ABD = p_3E + p_2 \\ A + B = CE \end{cases} \quad (5)$$

L'équation (4) peut s'écrire  $(4BCD - p_3)A = p_3B + p_2C$ . Si on pose  $F = 4BCD - p_3$  alors (4) est équivalent à

$$\begin{cases} FA = p_3B + p_2C \\ F + p_3 = 4BCD \end{cases} \quad (6)$$

La seconde équation montre que  $F \in \mathcal{A}$ , la première que  $F \in \mathcal{A}_+$ .

De plus, d'après (5) on a  $4(CE - B)BD = p_3E + p_2$  et donc  $(4BCD - p_3)E = 4B^2D + p_2$ . D'où

$$FE = 4B^2D + p_2 \quad (7)$$

## 2 Généralisation

### 2.1 Définitions

Comme pour les entiers, nous dirons qu'une fraction rationnelle est  $k$ -égyptienne si elle est la somme d'au plus  $k$  inverses de polynômes de  $\mathbb{Z}[X]$ .

On note  $\mathcal{A} = \mathbb{Z}[X]$  et  $\mathcal{A}_+$  l'ensemble des polynômes de  $\mathbb{Z}[X]$  dont le coefficient dominant est strictement positif. Les polynômes irréductibles de  $\mathcal{A}_+$  sont appelés des *éléments premiers*.

Dans l'anneau  $\mathcal{A}$ , le théorème fondamental de l'arithmétique est vérifié et le PGCD est unique si on lui impose d'appartenir à  $\mathcal{A}_+$ . On peut donc, sans rien changer ni à l'énoncé ni à la démonstration, réécrire la Proposition 1 dans ce nouveau contexte. Il en est de même pour les notations  $E$  et  $F$  ainsi que des relations associées.

### 2.2 Première application

PROPOSITION 2 (Théorème de Schinzel )

Soit  $a > 0$  et  $b$  tels que  $(a, b) = 1$ . Si  $4/(at + b)$  est 3-égyptienne<sup>4</sup> alors  $b$  est un non résidu quadratique modulo  $a$ .

---

3. Si on le souhaite, on peut poser  $x = T/A$ ,  $y = T/B$ ,  $z = T/C$  avec  $T = ABCD$ .

4.  $at + b$  est, par abus d'écriture, un polynôme (premier) de degré 1.

DÉMONSTRATION On pose  $p(t) = at + b$ . Il existe  $\tau$  tel que les polynômes  $p, A, B, C, D, E$  prennent des valeurs strictement positives pour  $t > \tau$ .

Suivant le cas, la relation  $4(B - CE)BD = p_3E + p_2$  s'écrit

$$4(CE - B)BD = E + p \quad \text{ou} \quad 4(CE - B)BD = pE + 1$$

c'est-à-dire

$$p = (4BCD - 1)E - 4B^2D \quad \text{ou} \quad pE^2 = (4BCDE - 1)E - 4B^2DE$$

d'où avec  $D' = DE$

$$p = -4B^2D \pmod{4BCD - 1} \quad \text{ou} \quad pE^2 = -4B^2D' \pmod{4BCD' - 1}$$

Si  $b$  est un résidu quadratique modulo  $a$ , il existe un entier  $k > \tau$  pour lequel  $ak + b$  est un carré. Pour  $t = k$ , on déduit des propriétés du symbole de Jacobi<sup>5</sup>

$$\left(\frac{p}{4BCD - 1}\right) = \left(\frac{-4B^2D}{4BCD - 1}\right) = -1$$

en contradiction avec le fait que  $p$  est un carré. Idem avec  $pE^2$ .

Détaillons le calcul. On pose  $D = 2^\alpha m$  avec  $m$  impair.

$$\left(\frac{-4B^2D}{4BCD - 1}\right) = -\left(\frac{D}{4BCD - 1}\right) = -\left(\frac{2}{4BCD - 1}\right)^\alpha \left(\frac{m}{4BCD - 1}\right)$$

Si  $\alpha > 0$  alors  $4ABCD - 1 = 7 \pmod{8}$  ce qui implique

$$\left(\frac{2}{4BCD - 1}\right) = 1$$

De plus, d'après la loi de réciprocité quadratique

$$\left(\frac{m}{4BCD - 1}\right) = (-1)^{(m-1)/2} \left(\frac{4BCD - 1}{m}\right) = (-1)^{(m-1)/2} \left(\frac{-1}{m}\right)$$

et donc

$$\left(\frac{m}{4BCD - 1}\right) = (-1)^{(m-1)/2} (-1)^{(m-1)/2} = 1$$

■

## 2.3 Equations modulaires

Pour alléger l'expression, on appellera *équation modulaire* une équation modulaire (ou un système d'équations modulaires) à *coefficients constants*.

Puisque  $A$  et  $B$  jouent des rôles symétriques on convient<sup>6</sup> que  $d^\circ B \leq d^\circ A$ , où  $d^\circ$  est le degré d'un polynôme.

LEMME 1 *Soit  $p$  un polynôme premier de degré 1.*

i) *Si la relation (1)  $4ABCD = A + B + pC$  est vérifiée alors*

$$d^\circ A = 1 \quad d^\circ B = 0 \quad d^\circ C = 0 \quad d^\circ D = 0 \quad (8a)$$

$$d^\circ A = 0 \quad d^\circ B = 0 \quad d^\circ C = 0 \quad d^\circ D = 1 \quad (8b)$$

$$d^\circ A = 1 \quad d^\circ B = 0 \quad d^\circ C = 1 \quad d^\circ D = 0 \quad (8c)$$

5. On note encore  $p, A, B, C, D, E$  les valeurs de ces polynômes pour  $t = k$ . Par ailleurs, un calcul analogue utilisant le symbole de Kronecker existe dans l'article de Yamamoto[6].

6. La définition arbitraire de  $F$  (factoriser  $A$  plutôt que  $B$ ) anticipe cette convention car sinon on aurait  $d^\circ F > 0$ .

ii) Si la relation (2)  $4ABCD = p(A + B) + C$  est vérifiée alors

$$d^\circ A = 0 \quad d^\circ B = 0 \quad d^\circ C = 0 \quad d^\circ D = 1 \quad (9a)$$

$$d^\circ A = 1 \quad d^\circ B = 0 \quad d^\circ C = 0 \quad d^\circ D = 1 \quad (9b)$$

$$d^\circ A = 1 \quad d^\circ B = 0 \quad d^\circ C = 1 \quad d^\circ D = 0 \quad (9c)$$

$$d^\circ A = 2 \quad d^\circ B = 1 \quad d^\circ C = 0 \quad d^\circ D = 0 \quad (9d)$$

DÉMONSTRATION La convention  $d^\circ B \leq d^\circ A$  implique  $d^\circ(A + B) = d^\circ A$ . De plus, comme  $CE = A + B$  alors  $d^\circ C \leq d^\circ A$

i) De la relation (1) on tire

$$(4ABD - p)C = A + B \quad (10)$$

et

$$(4BCD - 1)A = B + Cp \quad (11)$$

D'après (10), on a  $d^\circ(4ABD - p) \leq d^\circ A$  et donc  $d^\circ(4ABD - p) \leq d^\circ ABD$ .

\* Si  $d^\circ(4ABD - p) = d^\circ ABD$

De (10) on déduit

$$d^\circ ABD + d^\circ C = d^\circ A$$

c'est-à-dire

$$d^\circ B + d^\circ C + d^\circ D = 0$$

Avec (11) on en déduit

$$d^\circ A = d^\circ p = 1$$

\* Si  $d^\circ(4ABD - p) < d^\circ ABD$

On a alors

$$d^\circ ABD = d^\circ p = 1 \quad \text{et} \quad d^\circ(4ABD - p) = 0$$

De la première équation on déduit

$$d^\circ B = 0 \quad \text{et} \quad d^\circ A + d^\circ D = 1$$

De la seconde et de (10) on déduit

$$d^\circ C = d^\circ A$$

ii) De la relation (2) on tire

$$(4ABD - 1)C = p(A + B) \quad (12)$$

et

$$(4BCD - p)A = pB + C \quad (13)$$

De (12) on déduit

$$d^\circ ABD + d^\circ C = d^\circ A + d^\circ p$$

c'est-à-dire

$$d^\circ B + d^\circ C + d^\circ D = 1$$

Avec ici  $F = 4BCD - p$ , on a donc

$$d^\circ F \leq 1 \quad \text{et} \quad d^\circ(pB + C) = d^\circ pB$$

et d'après (13)

$$d^\circ F + d^\circ A = d^\circ B + 1$$

\* Si  $d^\circ F = 1$ , on a  $d^\circ A = d^\circ B$ . De plus, comme  $d^\circ F = 1$ , il existe  $t_0 \in \mathbb{R}$  tel que  $F(t_0) = 0$ . Puisque  $FE = 4B^2D + 1$ , alors  $4B^2(t_0)D(t_0) + 1 = 0$  et donc  $D(t_0) < 0$ . Par conséquent  $d^\circ D = 1$  et  $d^\circ B = d^\circ C = 0$ .

\* Si  $d^\circ F = 0$ , on a  $d^\circ A = d^\circ B + 1$ . ■

PROPOSITION 3 Soit  $p$  un polynôme premier de degré 1. La fraction  $4/p$  est 3-égyptienne si et seulement si l'une des 7 équations modulaires suivantes est vérifiée.

$$B + pC = 0 \pmod{4BCD - 1} \quad (14a)$$

$$p + E = 0 \pmod{4AB} \quad \text{et} \quad A + B = 0 \pmod{E} \quad (14b)$$

$$p + E + 4B^2D = 0 \pmod{4BDE} \quad (14c)$$

$$pE + 1 = 0 \pmod{4AB} \quad \text{et} \quad A + B = 0 \pmod{E} \quad (15a)$$

$$p + F = 0 \pmod{4BC} \quad \text{et} \quad pB + C = 0 \pmod{F} \quad (15b)$$

$$p + F = 0 \pmod{4BD} \quad \text{et} \quad 4B^2D + 1 = 0 \pmod{F} \quad (15c)$$

$$p + F = 0 \pmod{4CD} \quad \text{et} \quad p^2 + 4C^2D = 0 \pmod{F} \quad (15d)$$

avec  $(A, B) = (B, C) = (C, D) = (4ABD, E) = (4BCD, F) = 1$ .

DÉMONSTRATION Les [ ] font référence aux équations du Lemme précédent.

(14) Ici "(4) est équivalent à (5)" s'écrit

$$4ABCD = A + B + pC \iff (p + E = 4ABD \quad \text{et} \quad A + B = CE)$$

(14a) Cas [8a] :  $B, C, D$  sont constants. Dans le sens direct,  $(4BCD - 1)A = B + pC$ . D'où

$$B + pC = 0 \pmod{4BCD - 1}$$

Réciproquement, on pose

$$A = \frac{B + pC}{4BCD - 1}$$

(14b) Cas [8b] :  $A, B, E$  sont constants. Dans le sens direct, on a

$$p + E = 4ABD = 0 \pmod{4AB} \quad \text{et} \quad A + B = CE = 0 \pmod{E}$$

Réciproquement, on pose

$$D = \frac{p + E}{4AB} \quad \text{et} \quad C = \frac{A + B}{E}$$

(14c) Cas [8c] :  $B, D, E$  sont constants. Dans le sens direct,  $p + E = 4(CE - B)BD$ . D'où

$$p + E + 4B^2D = 4BDEC = 0 \pmod{4BDE}$$

Réciproquement, on pose

$$A = \frac{p + E}{4BD} \quad \text{et} \quad C = \frac{p + E + 4B^2D}{4BDE} \quad (CE = A + B)$$

(15) Ici "(4) est équivalent à (5)" s'écrit

$$4ABCD = p(A + B) + C \iff (4ABD = pE + 1 \quad \text{et} \quad A + B = CE)$$

et "(4) est équivalent à (6)" s'écrit

$$4ABCD = p(A + B) + C \iff (p + F = 4BCD \quad \text{et} \quad pB + C = FA)$$

avec  $F = 4BCD - p$  et  $FE = 4B^2D + 1$

(15a) Cas [9a] :  $A, B, E$  sont constants. Dans le sens direct on a

$$pE + 1 = 4ABD = 0 \pmod{4AB} \quad \text{et} \quad A + B = CE = 0 \pmod{E}$$

Réciproquement, on pose

$$D = \frac{pE + 1}{4AB} \quad \text{et} \quad C = \frac{A + B}{E}$$

Les cas suivants vérifient  $d^\circ A = d^\circ B + 1$  et donc  $d^\circ F = 0$ .

(15b) Cas [9b] :  $B, C, F$  sont constants. Dans le sens direct on a

$$p + F = 4BCD = 0 \pmod{4BC} \quad \text{et} \quad pB + C = FA = 0 \pmod{F}$$

Réciproquement, on pose

$$D = \frac{p + F}{4BC} \quad \text{et} \quad A = \frac{pB + C}{F}$$

(15c) Cas [9c] :  $B, D, F$  sont constants. Dans le sens direct on a

$$p + F = 4BCD = 0 \pmod{4BD} \quad \text{et} \quad 4B^2D + 1 = EF = 0 \pmod{F}$$

Réciproquement, on pose

$$C = \frac{p + F}{4BD} \quad E = \frac{4B^2D + 1}{F} \quad \text{et} \quad A = CE - B$$

On vérifie qu'alors  $FA = pB + C$ .

(15d) Cas [9d] :  $C, D, F$  sont constants. Dans le sens direct on a

$$p + F = 4BCD = 0 \pmod{4CD} \quad \text{et} \quad pB + C = FA = 0 \pmod{F}$$

Or

$$pB + C = p \frac{p + F}{4CD} + C = \frac{p^2 + pF + 4C^2D}{4CD}$$

Comme  $(4CD, F) = 1$ , on en déduit

$$p^2 + 4C^2D = 0 \pmod{F}$$

Réciproquement, on pose

$$B = \frac{p + F}{4CD} \quad \text{et} \quad A = \frac{pB + C}{F}$$

■

*Remarque* : Soit  $p$  un polynôme premier de degré 1. Le Lemme 1 démontre qu'il n'y a que 7 cas distincts de décompositions, la distinction se faisant sur les degrés respectifs de  $A, B, C, D$  ( $d^\circ B \leq d^\circ A$ ). Comme la Proposition 3 associe à chaque cas une équation modulaire, il n'existe donc que 7 équations modulaires à coefficients constants. Cela permet de construire un algorithme donnant l'ensemble (éventuellement vide) de toutes les décompositions de  $4/p$ .

## 2.4 Applications aux entiers

La démonstration de la Proposition 3 fournit des formules pour calculer  $A, B, C, D$ . Ces variables vérifient l'une des équations (1) ou (2) et prennent des valeurs strictement positives si les données le sont. D'où le corolaire suivant.

**COROLLAIRE 1** *Soit  $p$  un nombre premier impair. La fraction  $4/p$  est 3-égyptienne si et seulement si l'une des 7 équations modulaires de la Proposition 3 est vérifiée.*

Par la suite ces équations, aussi bien pour les polynômes que pour les entiers, seront désignées comme *équations de référence*.

### Comparaison avec les résultats antérieurs

Quatre de ces équations sont connues depuis longtemps, les autres sont nouvelles.

- Rosati [3] (1954) ne donne qu'une condition par type de décomposition. Bien qu'écrites sous une forme non modulaire ses équations (3) et (6) sont équivalentes à (14a) et (15a).
- Yamamoto [6] (1965) donne deux conditions par type de décomposition. Ecrite sous forme modulaire, ses équations (3) à (6) sont équivalentes (dans le désordre) à (14a), (14b), (15a), (15b).

Les polynômes nous permettent de comprendre pourquoi les équations équivalentes de Yamamoto donnent des résultats distincts. Bien mieux, ils nous donnent 3 nouvelles équations.

## Ensemble "complet" d'équations modulaires

Concernant les polynômes premiers de degré 1, les 7 équations de référence forment un ensemble complet<sup>7</sup>, c'est-à-dire que si une équation modulaire  $n = b \pmod{a}$  (avec  $(a, b) = 1$ ) est non équivalente à l'une des équations de référence alors  $4/(at + b)$  n'est pas une fraction 3-égyptienne. Cette propriété n'est pas conservée pour les entiers : il pourrait exister une méthode utilisant une telle équation et impliquant que  $4/n$  est une fraction 3-égyptienne. Mais, dans ce cas, elle devra nécessairement être d'un genre nouveau encore inconnu.

## 2.5 Exemples

**Exemple 0.** On retrouve bien sûr les identités du paragraphe 1.1. Ici, on cherche *uniquement* les décompositions de  $4/p$  données dans le paragraphe.

- $p = 3t - 1$  vérifie (14a) :  $p + 1 = 0 \pmod{3}$   
avec  $B = C = D = 1$ , ce qui donne  $A = (p + 1)/3 = t$ .
- $p = 4t - 1$  vérifie (14b) :  $p + 1 = 0 \pmod{4}$   
avec  $A = B = E = 1$  ce qui donne  $C = 2$  et  $D = (p + 1)/4 = t$ .
- $p = 8t - 3$  vérifie (14b) :  $p + 3 = 0 \pmod{8}$   
avec  $A = 1$ ,  $B = 2$ ,  $E = 3$  ce qui donne  $C = 1$  et  $D = (p + 3)/8 = t$ .

**Exemple 1.**  $p = 24 \cdot 5t - 23$  ( $p = 1 \pmod{24}$  et  $p = 2 \pmod{5}$ )

On donne toutes les décompositions de  $4/p$  et la particularité est que les 7 sous types (indiqués entre []) sont représentés. On ne connaît pas d'autre exemple analogue vérifiant  $p = 1 \pmod{24}$ .

$$[14a] \quad \frac{4}{p} = \frac{1}{p} \left( \frac{1}{4} + \frac{1}{4(16t-3)} \right) + \frac{1}{2(16t-3)}$$

$$[14b] \quad \frac{4}{p} = \frac{1}{p} \left( \frac{1}{10(6t-1)} + \frac{1}{2(6t-1)} \right) + \frac{1}{5(6t-1)}$$

$$[14c] \quad \frac{4}{p} = \frac{1}{p} \left( \frac{1}{10t} + \frac{1}{10t(6t-1)} \right) + \frac{1}{5(6t-1)}$$

$$\frac{4}{p} = \frac{1}{p} \left( \frac{1}{2t} + \frac{1}{2t(15t-1)} \right) + \frac{1}{2(15t-1)}$$

$$[15a] \quad \frac{4}{p} = \frac{1}{5(21t-4)} + \frac{1}{2(21t-4)} + \frac{1}{10(21t-4)p}$$

$$[15b] \quad \frac{4}{p} = \frac{1}{5(6t-1)} + \frac{1}{2(6t-1)(100t-19)} + \frac{1}{10(6t-1)(100t-19)p}$$

$$\frac{4}{p} = \frac{1}{5(6t-1)} + \frac{1}{10(6t-1)(20t-3)} + \frac{1}{2(6t-1)(20t-3)p}$$

$$\frac{4}{p} = \frac{1}{2(15t-1)} + \frac{1}{(15t-1)(16t-3)} + \frac{1}{2(15t-1)(16t-3)p}$$

$$[15c] \quad \frac{4}{p} = \frac{1}{5(6t-1)} + \frac{1}{10(6t-1)(21t-4)} + \frac{1}{10(21t-4)p}$$

$$[15d] \quad \frac{4}{p} = \frac{1}{5(6t-1)} + \frac{1}{10(120t^2-43t+4)} + \frac{1}{10(6t-1)(120t^2-43t+4)p}$$

**Exemple 2.** Dans cet exemple, chaque  $p$  est de la forme  $p = 24 \cdot 583t + b$ . A l'opposé de l'exemple 1, la particularité est que, pour certains  $b$ ,  $4/p$  n'admet qu'une seule décomposition. Une valeur de  $b$  est donnée pour chaque sous type.

---

7. De plus l'exemple 2 ci-dessous montre que ces équations sont indépendantes.



$$[14a] \quad p = 24 \cdot 583t - 911 \quad (p = 1 \pmod{24} \quad \text{et} \quad p = 255 \pmod{583})$$

$$\frac{4}{p} = \frac{1}{p} \left( \frac{1}{2 \cdot 73} + \frac{1}{6(16t-1)} \right) + \frac{1}{3 \cdot 73(16t-1)}$$

$$[14b] \quad p = 24 \cdot 583t - 119 \quad (p = 1 \pmod{24} \quad \text{et} \quad p = 464 \pmod{583})$$

$$\frac{4}{p} = \frac{1}{p} \left( \frac{1}{66t} + \frac{1}{53t} \right) + \frac{1}{66 \cdot 53t}$$

$$[14c] \quad p = 24 \cdot 583t - 1127 \quad (p = 1 \pmod{24} \quad \text{et} \quad p = 39 \pmod{583})$$

$$\frac{4}{p} = \frac{1}{p} \left( \frac{1}{22t} + \frac{1}{2t(159t-11)} \right) + \frac{1}{22(159t-11)}$$

$$[15a] \quad p = 24 \cdot 583t - 1799 \quad (p = 1 \pmod{24} \quad \text{et} \quad p = 533 \pmod{583})$$

$$\frac{4}{p} = \frac{1}{50 \cdot 1749(70t-9)} + \frac{1}{50(70t-9)} + \frac{1}{1749(70t-9)p}$$

$$[15b] \quad p = 24 \cdot 583t - 11159 \quad (p = 1 \pmod{24} \quad \text{et} \quad p = 501 \pmod{583})$$

$$\frac{4}{p} = \frac{1}{22(159t-125)} + \frac{1}{8(242t-193)(159t-125)} + \frac{1}{88(242t-193)(159t-125)p}$$

$$[15c] \quad p = 24 \cdot 583t - 503 \quad (p = 1 \pmod{24} \quad \text{et} \quad p = 80 \pmod{583})$$

$$\frac{4}{p} = \frac{1}{6 \cdot 583t} + \frac{1}{6 \cdot 53t(306t-11)} + \frac{1}{583(306t-11)p}$$

$$[15d] \quad p = 24 \cdot 583t - 6407 \quad (p = 1 \pmod{24} \quad \text{et} \quad p = 6 \pmod{583})$$

$$\begin{aligned} \frac{4}{p} = \frac{1}{22(159t-71)} + \frac{1}{22(13992t^2-12655t+2861)} \\ + \frac{1}{11(159t-71)(13992t^2-12655t+2861)p} \end{aligned}$$

### 3 Crible modulaire

Les algorithmes donnant, pour un entier  $n > 2$ , au moins une décomposition (voire toutes) de  $4/n$  ont leur intérêt. Cependant, en ce qui concerne la vérification de la conjecture, un algorithme efficace nécessite un autre point de vue<sup>8</sup>.

On note  $\mathbb{N}_0$  l'ensemble des entiers  $n \in \mathbb{N}$  vérifiant la condition  $n = 1 \pmod{24}$ . La méthode décrite ci-après tient compte expressément du fait que les nombres testés appartiennent à  $\mathbb{N}_0$ . Par ailleurs, on abandonne la condition  $n$  premier, la vérification préalable étant trop coûteuse en temps de calcul. Pour le polynôme  $at + b$ , les conditions correspondantes sont  $at + b = 1 \pmod{24}$  (ce qui est équivalent à  $a = 0 \pmod{24}$  et  $b = 1 \pmod{24}$ ) et l'abandon de la condition  $(a, b) = 1$ .

#### 3.1 Filtres modulaires

*Définition :* Un *crible* est un ensemble ordonné de filtres.

*Définition :* Un *filtre*<sup>9</sup> modulo  $m$  est un ensemble  $F$  tel que pour tout  $n \in \mathbb{N}_0$

$$n \% m \in F \Rightarrow 4/n \text{ est 3-égyptienne}$$

<sup>8</sup>. Ce point de vue est utilisé dès l'article de Rosati et lui est même peut être antérieur.

<sup>9</sup>. On reprend la terminologie imagée employée par Swett. Les entiers  $n \in \mathbb{N}_0$  tels que  $n \% m \in F$  vérifient la conjecture et sont "retenus" par le filtre, les autres "passent au travers".

où  $n \% m$  désigne le résidu de  $n$  modulo  $m$  (notation empruntée au langage C).

Pour  $a > 0$ , on note  $\Omega_a$  l'ensemble des  $b \in \mathbb{Z}$  tels que  $4/(at + b)$  est 3-égyptienne. Pour  $m$  impair, on pose  $S_m = (\Omega_{[m,24]} \cap \mathbb{N}_0) \% m$  où  $[u, v]$  désigne le plus petit commun multiple de  $u$  et  $v$ . Les propriétés suivantes sont immédiates.

- i) Si  $q \mid a$  alors  $\Omega_q \subset \Omega_a$ .
- ii) Si  $b_1 = b_2 \pmod{a}$  alors  $b_1 \in \Omega_a \Rightarrow b_2 \in \Omega_a$ .
- iii) Si  $n \in \Omega_a$  ( $n > 0$ ) alors  $4/n$  est 3-égyptienne.
- iv) Si  $n \in \mathbb{N}_0$  alors  $(n \in \Omega_{[m,24]} \iff n \% m \in S_m)$ , ce qui montre que  $S_m$  est un filtre modulo  $m$ .
- v) Si  $n \in \mathbb{N}_0$  et si  $q \mid m$  alors  $n \% q \in S_q \Rightarrow n \% m \in S_m$ .

*Définition* : On dit que  $n \in \mathbb{N}_0$  est *certifié* si il existe  $m$  tel que  $n \% m \in S_m$ . On dit alors que  $n$  est certifié par  $m$  ou que  $m$  est un *certificat modulaire* de  $n$  (vocabulaire emprunté à la théorie de la complexité).

*Les premiers résultats avec  $m > 3$  premier :*

$$\begin{array}{ll}
S_5 = \{0, 2, 3\} & S_{19} = \{0, 8, 12, 14, 15, 18\} \\
S_7 = \{0, 3, 5, 6\} & S_{23} = \{0, 7, 10, 11, 15, 17, 19, 20, 21, 22\} \\
S_{11} = \{0, 7, 8, 10\} & S_{29} = \{0, 14, 18, 19, 21, 26, 27\} \\
S_{13} = \{0, 5, 6, 8, 11\} & S_{31} = \{0, 15, 22, 23, 24, 27, 29, 30\} \\
S_{17} = \{0, 10, 11, 12, 14\} & S_{37} = \{0, 5, 15, 18, 22, 23, 29, 32, 35\}
\end{array}$$

*Quelques résultats avec  $m$  composé impair :*

$$\begin{array}{l}
S_{15} = \{7, 10, 13\} \\
S_{35} = \{0, 2, 3, 5, 6, 7, 8, 10, 12, 13, 14, 15, 17, 18, 19, 20, 21, 22, 23, 24, \\
\quad 25, 26, 27, 28, 30, 31, 32, 33, 34\} \\
S_{55} = \{0, 2, 3, 5, 7, 8, 10, 11, 12, 13, 15, 17, 18, 19, 20, 21, 22, 23, \\
\quad 24, 25, 27, 28, 29, 30, 32, 33, 35, 37, 38, 39, 40, 41, 42, 43, \\
\quad 44, 45, 47, 48, 50, 51, 52, 53, 54\}
\end{array}$$

### 3.2 Filtres réduits

Si  $m$  est composé, certains entiers  $n \in \mathbb{N}_0$  sont certifiés à la fois par  $m$  et par l'un de ses diviseurs (cf. la propriété v) ci dessus). Pour déterminer ce qui est propre à  $m$ , on introduit la notation suivante.

*Définition* : Le *filtre réduit*  $S_m^*$  est l'ensemble des  $x \in S_m$  tels que

$$x \% q \notin S_q \text{ pour tout } q \mid m, q \neq m$$

*Remarque* : Si  $m$  est premier alors  $S_m^* = S_m$ .

*Les premiers résultats (non vides) avec  $m$  composé*

$$\begin{array}{ll}
S_{55}^* = \{24, 39\} & S_{95}^* = \{29, 59, 79, 89\} \\
S_{65}^* = \{54, 59\} & S_{99}^* = \{61, 79, 94\} \\
S_{77}^* = \{46, 72\} & S_{117}^* = \{85, 106\} \\
S_{85}^* = \{54, 74\} & S_{119}^* = \{23, 39, 57, 58, 71, 88, 107, 109\}
\end{array}$$

## 4 Vérification de la conjecture

### 4.1 Choix des progressions

Les entiers testés sont en progression arithmétique et, plus précisément, sont de la forme  $n = 24k+1$ . Le pas de la progression est ici  $G_0 = 24$  mais, en utilisant quelques filtres  $S_m$ , on peut obtenir des progressions dont le pas est plus grand.

En utilisant  $S_5 = \{0, 2, 3\}$  on ne teste que les entiers  $n$  vérifiant

$$n \% 24 = 1 \quad \text{et} \quad n \% 5 \in \{1, 4\}$$

c'est-à-dire, à l'aide du théorème des restes chinois

$$n \% 120 \in \{1, 49\}$$

Le pas est  $G_1 = 120$ , pour un nombre de résidus égal à 2 : le pas moyen est donc  $g_1 = 60$ . Par rapport à 24, on teste donc 2.5 fois moins d'entiers ( $60/24 = 2.5$ ).

En utilisant en plus  $S_7 = \{0, 3, 5, 6\}$  on ne teste que les entiers  $n$  vérifiant

$$n \% 120 \in \{1, 49\} \quad \text{et} \quad n \% 7 \in \{1, 2, 4\}$$

c'est-à-dire

$$n \% 840 \in R_2$$

où  $R_2 = \{1, 121, 169, 289, 361, 529\}$  est l'ensemble des résidus<sup>10</sup>. Le pas est  $G_2 = 840$  et le pas moyen  $g_2 = 140$ . Par rapport à 24, on teste presque 6 fois moins d'entiers ( $140/24 = 35/6$ ).

On peut continuer le processus et utiliser d'autres  $S_m$ . Les entiers testés sont alors de la forme

$$n \% G_i \in R_i$$

où les premières valeurs de  $G_i = G_{i-1}m_i$  et  $\#R_i$  (le nombre d'éléments de  $R_i$ ) sont données dans le tableau ci-dessous.

| $i$ | $m_i$ | $G_i$       | $\#R_i$ | $g_i$ |
|-----|-------|-------------|---------|-------|
| 1   | 5     | 120         | 2       | 60    |
| 2   | 7     | 840         | 6       | 140   |
| 3   | 11    | 9 240       | 34      | 272   |
| 4   | 13    | 120 120     | 192     | 626   |
| 5   | 17    | 2 042 040   | 1 507   | 1 355 |
| 6   | 19    | 38 798 760  | 13 380  | 2 900 |
| 7   | 23    | 892 371 480 | 147 348 | 6 056 |

Ce tableau appelle trois remarques.

- La première concerne la réduction des  $R_i$  (effectuée dans le tableau). Si  $n = r \pmod{G_i}$  alors pour tout  $q$  diviseur de  $G_i$  on a  $n \% q = r \% q$ , ce qui permet d'éliminer les éléments  $r \in R_i$  vérifiant  $r \% q \in S_q$ . Cette réduction est essentielle, sinon la procédure est une complication inutile.
- La seconde concerne la dernière colonne : le pas moyen  $g_i = G_i / \#R_i$  est un bon indicateur de rapidité. Par exemple, comme  $6\,056/140 \approx 43$ , la méthode associée à  $G_7$  teste environ 43 fois moins d'entiers que celle associée à  $G_2 = 840$ , ce qui réduit d'autant le temps de calcul.
- La dernière concerne le choix des  $m_i$ . L'ordre usuel est trompeur : tout autre ensemble de 7 nombres donne, semble-t-il, un  $g_7$  inférieur. Pour 8 nombres il faut vraisemblablement ajouter 31 (et non 29). Ces deux affirmations sont cependant à vérifier.

---

10. C'est le choix retenu par Swett.

## 4.2 Crible optimisé

On note  $\mathbb{N}_i$  l'ensemble des entiers  $n \in \mathbb{N}$  vérifiant  $n \% G_i \in R_i$ . Ce qui précède montre que tout entier n'appartenant pas à  $N_i$  vérifie la conjecture.

Soit  $N = 10^{17}$  et  $M$  l'ensemble des nombres impairs  $m < 5000$ . L'expérience montre que tout  $n \in \mathbb{N}_7$  possède un certificat modulaire dans  $M$  si  $n < N$  et si  $n$  n'est pas un carré. En terme de recouvrement, il est équivalent de dire que  $\mathbb{N}_7 \setminus \bigcup_{m \in M} \Omega_{[m, 24]}$  ne contient aucun élément  $n < N$ , hormis des carrés.

On pourrait utiliser cet ensemble pour démontrer que la conjecture est vérifiée jusqu'à l'ordre indiqué. Cependant si l'on veut que le temps de calcul soit le plus court possible, il est souhaitable d'optimiser le crible c'est-à-dire de supprimer les éléments inutiles et d'ordonner  $M$  afin d'avoir au début les filtres les plus efficaces<sup>11</sup>. Par exemple pour  $N = 10^{17}$ , notre programme en C++ utilise le crible défini par l'ensemble ordonné  $M = MOD$  ci-dessous.

$MOD = \{3, 5, 7, 11, 13, 17, 19, 23, 4495, 2491, 2627, 4661, 4223, 1505, 4355, 3355, 4509, 4775, 2629, 4565, 4599, 4585, 3955, 3535, 3857, 3115, 3419, 3949, 3395, 3353, 1391, 1199, 3775, 4325, 4031, 2799, 1639, 4475, 2159, 4795, 2961, 1727, 4075, 1791, 4743, 2849, 3595, 1115, 3445, 3263, 2155, 2065, 2515, 2681, 4195, 3223, 2519, 4103, 3731, 4345, 3743, 2439, 1055, 2951, 1799, 4193, 1991, 3047, 2933, 3951, 4147, 1631, 2219, 4615, 3913, 3679, 1535, 2959, 1655, 4123, 1439, 3839, 1319, 3695, 4255, 3895, 1351, 2495, 1835, 2855, 2335, 4529, 1917, 1079, 1559, 1735, 1679, 2165, 4367, 4555, 2359, 2723, 3065, 3899, 3295, 3035, 4927, 3359, 4437, 3635, 4315, 2735, 3241, 4319, 4105, 4069, 1039, 4059, 1247, 3095, 4571, 3665, 1007, 1583, 4895, 1847, 2435, 1765, 2807, 3647, 1343, 2651, 3965, 1511, 2655, 4403, 1151, 887, 2935, 3545, 2879, 1967, 2815, 2399, 4419, 1159, 4487, 3119, 1223, 2039, 4745, 2305, 1103, 4077, 3215, 3715, 2279, 4915, 4873, 1031, 1475, 3865, 2483, 1399, 1823, 3173, 3305, 2241, 3985, 3563, 1349, 1259, 3959, 4415, 3455, 2615, 1487, 3599, 3935, 1759, 3505, 1871, 4879, 4535, 3199, 2045, 1367, 1493, 1919, 3787, 2111, 1975, 2053, 4739, 1231, 4151, 1837, 1213, 3655, 2183, 4135, 4939, 1019, 3023, 3995, 1855, 4265, 4079, 3983, 2575, 1063, 2351, 4985, 2687, 3167, 2447, 2725, 4631, 4595, 4115, 4175, 4055, 4679, 1013, 2239, 4385, 1091, 3429, 1909, 1719, 2365, 3415, 3079, 4955, 1147, 1133, 3191, 3475, 2759, 4405, 2207, 4765, 3431, 1139, 4471, 2727, 4145, 3247, 1279, 1751, 3755, 1087, 4835, 1733, 4645, 1979, 4711, 1177, 1073, 3055, 3239, 2999, 2087, 4855, 4039, 1703, 3527, 4295, 4799, 4207, 4505, 1187, 1109, 1567, 1379, 2119, 2911, 2591, 2015, 3785, 1651, 3155, 1819, 4751, 3719, 4735, 2345, 2831, 2099, 4995, 1427, 2059, 1333, 1069, 1663, 2719, 2063, 4285, 2231, 1093, 1607, 1423, 1411, 1027, 3805, 1769, 1121, 1903, 4063, 4759, 1363, 1973, 4715, 2663, 3863, 1433, 2479, 4703, 3299, 1451, 2339, 1613, 1471, 1619, 3671, 2287, 2367, 3845, 3537, 1591, 3733, 4463, 1271, 1931, 4619, 2903, 2135, 4921, 4685, 4705, 1003, 1429, 1193, 4067, 3275, 4311, 1327, 3015, 1499, 2413, 1237, 1181, 4045, 4081, 3605, 3779, 3103, 2837, 1579, 3439, 1033, 3799, 2333, 1829, 1241, 4393, 2357, 4159, 2699, 3791, 2453, 3625, 2579, 4945, 4127, 1649, 4741, 4871, 1667, 2177, 3835, 1043, 3407, 4919, 4885, 2267, 2693, 2507, 4967, 2327, 4639, 1691, 1549, 2583, 1123, 1717, 1999, 1807, 1933, 4553, 1049, 3479, 1553, 1853, 2543, 4343, 1501, 2743, 3699, 1787, 3989, 1129, 1525, 4445, 1675, 1993, 1301, 2273, 1217, 1843, 4003, 2411, 3245, 3401, 1117, 1789, 3379, 3901, 1831, 1957, 4085, 1507, 1987, 3373, 3893, 1621, 1943, 3937, 1291, 1543, 1571, 2143, 2533, 2767, 3253, 4883, 2551, 2833, 1229, 1877, 1949, 2009, 4391, 1643, 2251, 2729, 3915, 1907, 2243, 2603, 2669, 2897, 3043, 3313, 3739, 1171, 1361, 1817, 1879, 2659, 3623, 4283, 4859, 1537, 2003, 2161, 2389, 2869, 4439, 1099, 1415, 2269, 2293, 2943, 3233, 3967, 4181, 4261, 4559, 4699, 1447, 1895, 1921, 2195, 2939, 3293, 3565, 3607, 3749, 4247, 4591, 4829, 1157, 1417, 1951, 1997, 2179, 2225, 2619, 2785, 3041, 3717, 4583, 4783, 4887, 1283, 1517, 1721, 1747, 1961, 2033, 2117, 2129, 2741, 2803, 2893, 3161, 3589, 3613, 1211, 1273, 1459, 1483, 1811, 1867, 1889, 1971, 2043, 2069, 2149, 2213, 2423, 2709, 2779, 3013, 3149, 3551, 4013, 4097, 4363, 4399, 4589, 4681, 1021, 1097, 1145, 1197, 1297, 1373, 1397, 1555, 1609, 1723, 1773, 1777, 1783, 1801, 2123, 2191, 2259, 2291, 2371, 2407, 2443, 2671, 2845, 3389, 3493, 3725, 4021, 4171, 4351, 4999\}$

## 4.3 Résultats

Les entiers testés sont de la forme  $n = r + k \times G_7$  avec  $r \in R_7$  et  $0 \leq k < K$ . Pour  $N = 10^{17}$ , on prend  $K = 112\,066\,560$ , ce qui donne  $16\,512\,783\,482\,880$  entiers dont  $51\,732\,427$  carrés.

11. Les filtres réduits servent de base à une approche essentiellement expérimentale.
